# Supplementary material for: Sampling-based Fast Gradient Rescaling Method for Highly Transferable Adversarial Attacks
Source: arXiv:2307.02828 source file (2023-07-06)
Supplement: Supplementary file 1 [file 06Appendix.tex]

%\newpage 

We conduct ablation studies to investigate the effectiveness of our \emph{rescale} function on the Inc-v3 model without input transformations.
We also compare with the staircase sign method~\cite{gao2021staircase}, termed S$^2$M, which is a recent work that also focuses on the improvement of the \emph{sign} function. 
This method heuristically divides the gradient sign into several segments according to the sorted values of the gradient units, and then assigns each segment with a staircase weight for better crafting adversarial perturbation. Specifically, it assigns the staircase weights according to the $p$-th percentile of the gradient units at each iteration where $p$ depends on the number $K$ of staircases.

We carry out experiments to test the \emph{rescale} function compared with I-FGSM (left) and I-FGS$^2$M (right) as illustrated in Fig.~\ref{fig:srescale}. The results show that our method is much more effective on both single and ensemble models.

We then conduct an ablation study to investigate each component of our method, 
and continue to compare with I-FGS$^2$M~\cite{gao2021staircase}.
We test our method and I-FGS$^2$M in the multi-step case to compare with I-FGSM, and the results are shown in Table~\ref{tab:FGRM}. 
We can observe that our I-FGRM exhibits clearly better results as compared with I-FGSM, 
%and after adding the sampling, our final S-FGRM gains further improvement on I-FGRM. 
and could perform nearly the same results as compared with I-FGS$^2$M~\cite{gao2021staircase}. After adding the depth first sampling method, our SI-FGRM gains further improvement on I-FGRM, and outperforms I-FGS$^2$M~\cite{gao2021staircase} significantly. 

\begin{figure}[htbp]
    \centering
    \begin{minipage}[c]{0.23\textwidth}
        \centering
        %\vspace{1.05cm}
        \includegraphics[width=0.85\linewidth]%[width=0.75\linewidth]
        {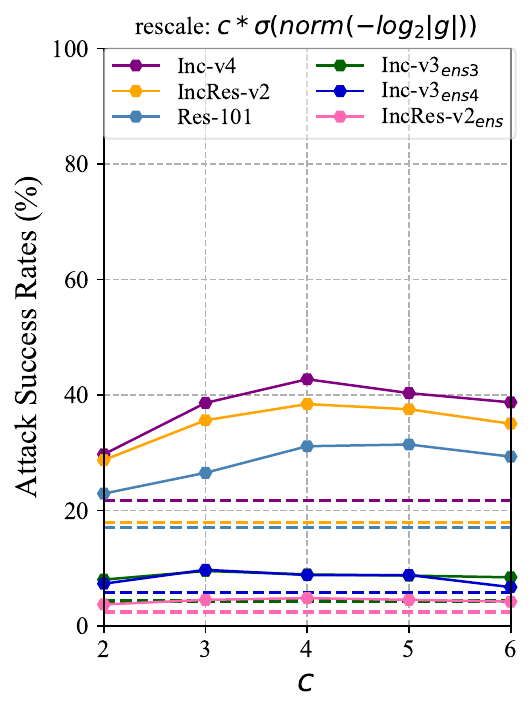}
        %\subcaption{(a)SMI-FGRM}
        \label{subfig:cmpFGSM}
    \end{minipage}
    %\hspace{0.05cm}
    \begin{minipage}[c]{0.23\textwidth}%{0.45\textwidth}
        \centering
        \includegraphics[width=0.85\linewidth]{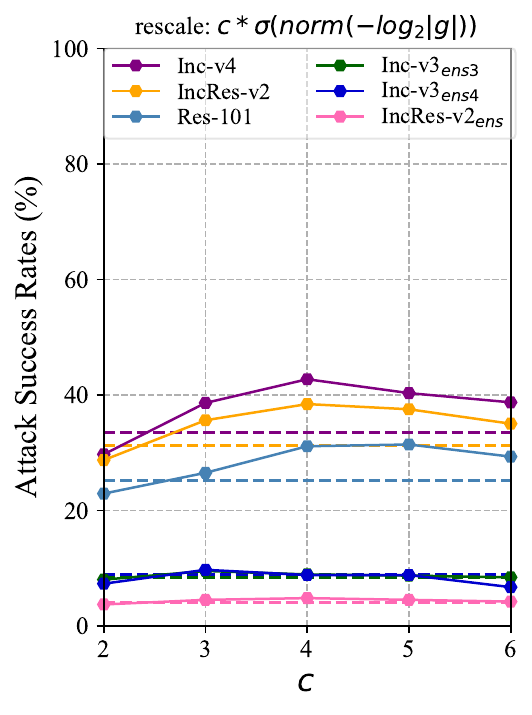}
        %\subcaption{(b)SNI-FGRM}
        \label{subfig:cmpS2M}
    \end{minipage}
    \caption{The attack success rates (\%) on six models with adversarial examples generated by Inc-v3 for various scale factors of $c$. The dashed lines represent the vanilla method of I-FGSM on the left and I-FGS$^2$M with their best settubg of $k = 64$ for Staircase on the right.}
    \label{fig:srescale}
    % \vspace{-0.5em}
\end{figure}

Note that our method is more efficient than Staircase~\cite{gao2021staircase} because we do not need to sort the gradient values to calculate the percentile. 
Considering the batch input whose size is $S = B\times H\times W\times C$, where $B$ is the batch size and $H$, $W$, $C$ represent the height, width and channel of an image, the Staircase method needs $O(S\log S)$ computational cost per iteration while our rescale method only needs $O(S)$. And in most cases, our attack success rate can exceed Staircase, as illustrated on the right of Fig.~\ref{fig:srescale}. As shown in the results, when attacking the ensemble models, the difference in attack success rate is indistinct for I-FGRM and I-FGS$^2$M. Still, both methods can improve significantly against the vanilla I-FGSM, justifying our assumption in the motivation subsection. 
%whose time complexity is only $O(H\times W\times C)$.% 

% \input{tab/C_I}

% \input{tab/C_MI}

% \input{tab/C_MI_CT}
